# Supplementary material for: The nuclear contacts and short range correlations in nuclei
Source: arXiv:1612.00923 source file (2018-01-22)
Supplement: Supplementary file 1 [file Supplementary_Materials_v5.pdf]

# Supplemental Materials: The nuclear contacts and short range correlations in nuclei

## THE UNIVERSAL TWO-BODY FUNCTIONS AND THE CONTACTS

In the paper we have used the two-body wave functions in momentum and coordinate space, $\tilde{\varphi}_\alpha(\boldsymbol{k}_{ij})$ and $\varphi_\alpha(\boldsymbol{r}_{ij})$, to extract the values of the nuclear contacts from two-body densities. These functions are defined as the zero-energy solution of the two-body nuclear problem for the channel $\alpha$. The channel $\alpha$ includes the orbital angular momentum $\ell$, the spin $s$ and the total angular momentum of the pair $j$ and its projection $m$. The index $ij$ corresponds to $pn$, $pp$, and $nn$ pairs. The $\varphi_\alpha(\boldsymbol{r}_{ij})$ and $\tilde{\varphi}_\alpha(\boldsymbol{k})$ functions are "universal" in the sense that they are the same for all nuclei.

The functions used in this work were calculated numerically using the AV18 potential for zero energy. The obtained wave functions are insensitive to the exact value of the energy for small distances and large momenta. The calculated functions are presented in Figs. S1 and S2 in coordinate and momentum space, respectively.

The definition of the contacts used in this work is slightly different than the original definition of the nuclear contacts of Ref. [S1]. First, here we used the definition $C_{ij}^{\alpha\alpha} = N_{ij}\langle A_{ij}^{\alpha}|A_{ij}^{\alpha}\rangle$, where $N_{ij}$ is the number of $ij$ pairs, without the $16\pi^2$ factor of the original definition. We also assumed that the contacts are averaged over the nuclear magnetic projection. Additionally, the deuteron-channel contact $C_{pn}^{s=1}$ is the sum over the three diagonal deuteron contacts with different pair magnetic projection $m = \pm 1, 0$.

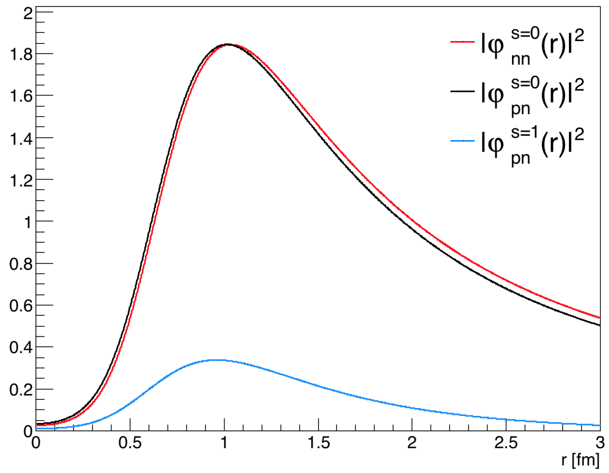


FIG. S1. The two-body universal functions in coordinate space as calculated using the AV18 potential.

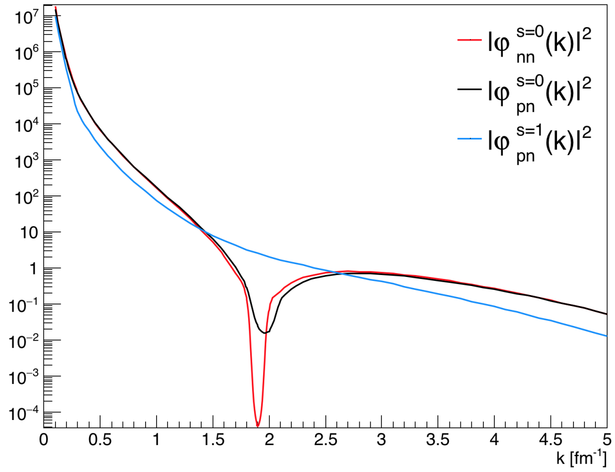


FIG. S2. The two-body universal functions in momentum space as calculated using the AV18 potential.

## EXAMPLE OF THE CONTACT FITTING

As explained in the paper, the nuclear contacts were extracted by fitting the two-body densities of the VMC calculations [S2]. An example of the fitting is presented in Figs. S3 and S4 for $^{10}$B, in coordinate and momentum space, respectively. In momentum space, the uncertainties of the resulting contacts are obtained by varying the fit limits by $\pm 0.2$ fm$^{-1}$. In coordinate space, the uncertainties are obtained by varying the fit limits by $\pm 0.25$ fm.

## THE ONE-BODY MOMENTUM DISTRIBUTION

After extracting the values of the contacts using the two-body densities, we can check the relation between the contacts and the one-body momentum distribution. In the paper, this relation was verified for $^4$He using the values of the contacts extracted in momentum space. Here we present the results for all of the available nuclei in the VMC calculations, using both the contact values extracted in coordinate and momentum space. See Figs. S5 - S18, where the neutron momentum distribution of the VMC results is compared to the contact expression.

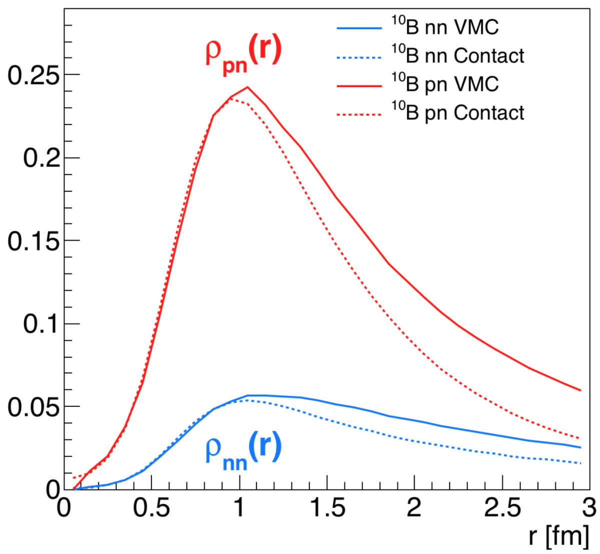


FIG. S3. Extraction of the $^{10}$B contacts from the two-body densities in coordinate space using the VMC results

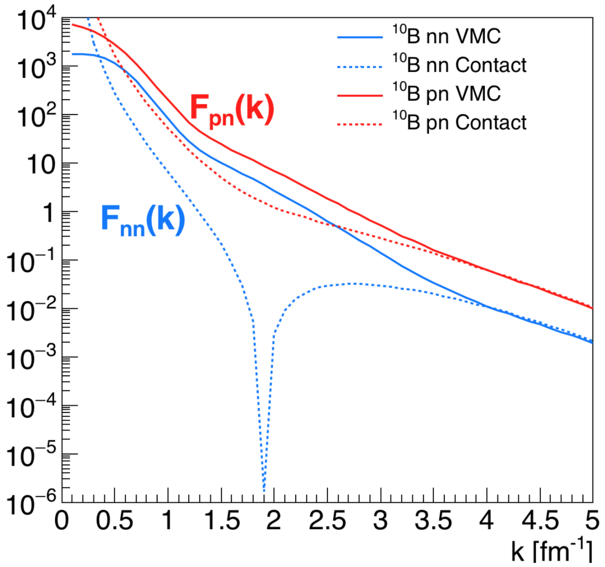


FIG. S4. Extraction of the $^{10}$B contacts from the two-body densities in momentum space using the VMC results

## PROTON-PROTON TO NEUTRON-PROTON RATIO

The ratio between the number of *pp* SRC pairs to the number of *np* SRC pairs, as a function of the relative momentum $k$, can be calculated using the values of the contacts and the two-body universal functions. In the paper, this ratio was presented for $^4$He, and compared to experimental data. Here, in Fig. S19, we present the same ratio for $^{12}$C, and compare to the experimental data of Ref. [S3].

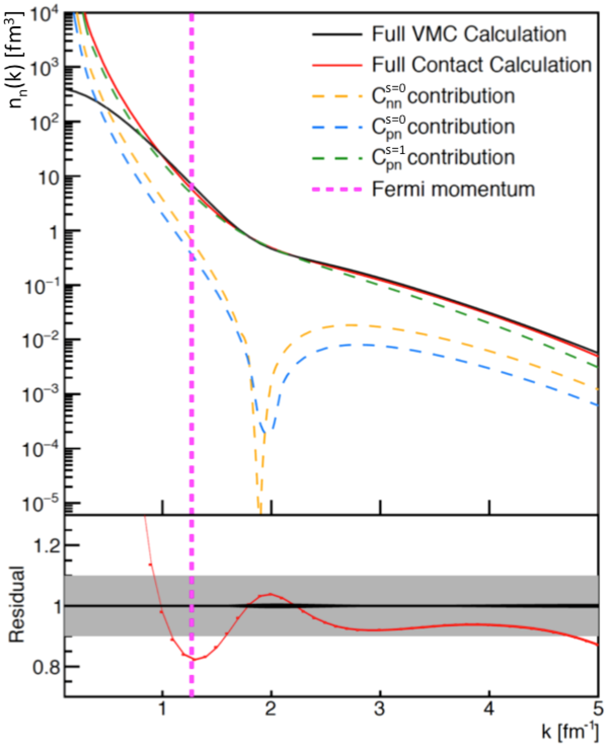


FIG. S5. The $^4$He neutron momentum distribution is reconstructed using the contact values extracted in coordinate space, and compared to the VMC data

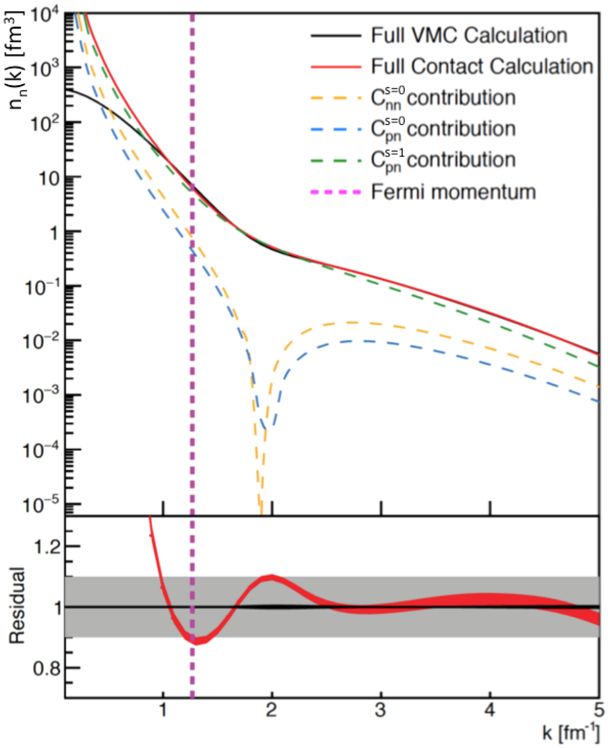


FIG. S6. The $^4$He neutron momentum distribution is reconstructed using the contact values extracted in momentum space, and compared to the VMC data

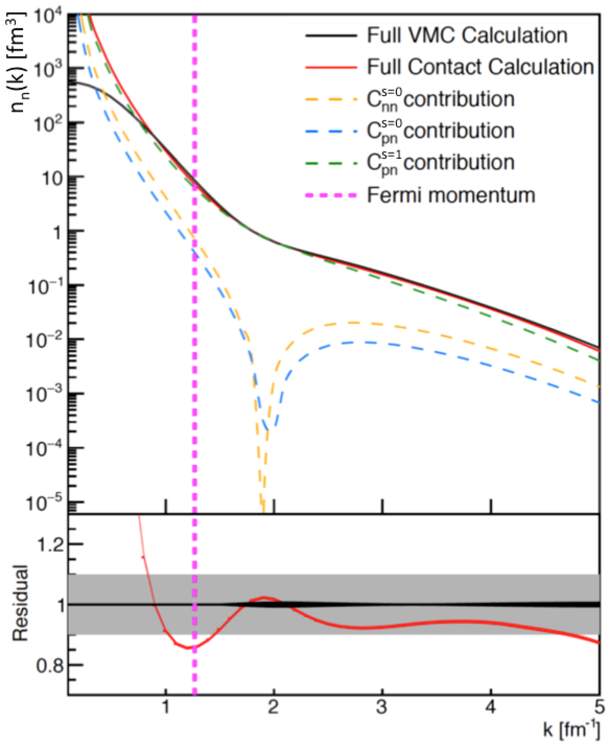


FIG. S7. The $^6$Li neutron momentum distribution is reconstructed using the contact values extracted in coordinate space, and compared to the VMC data

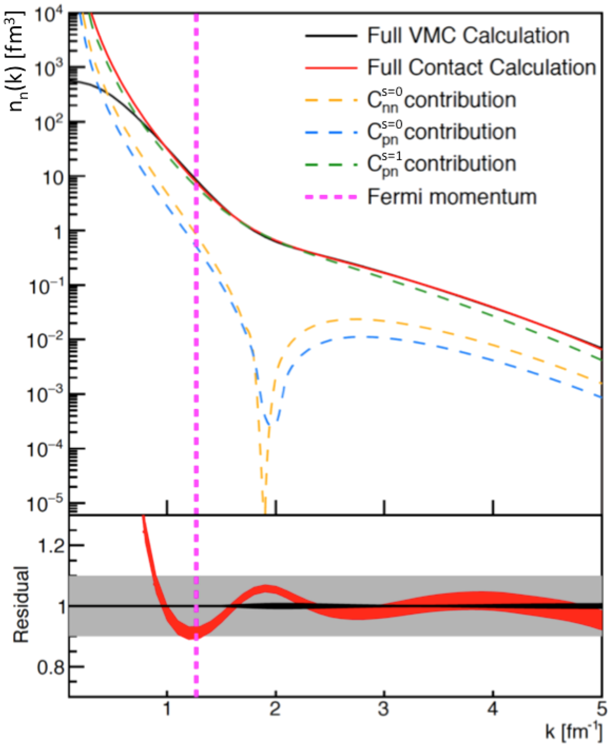


FIG. S8. The $^6$Li neutron momentum distribution is reconstructed using the contact values extracted in momentum space, and compared to the VMC data

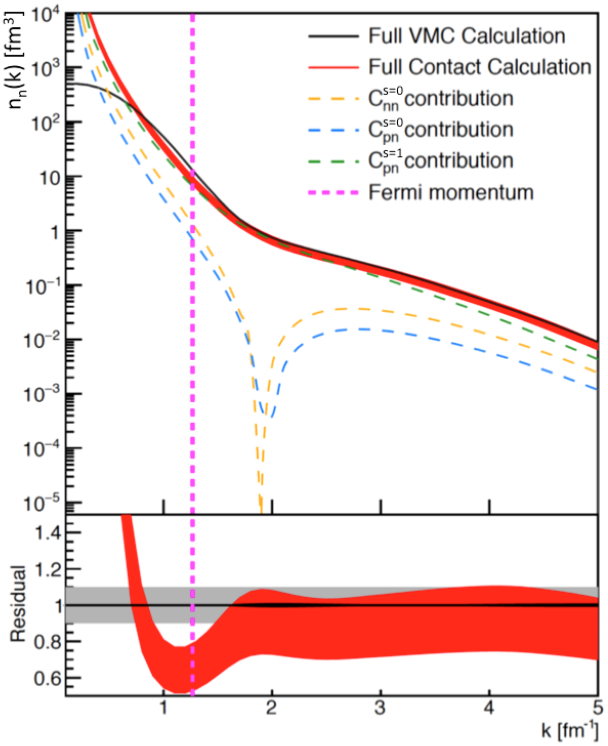


FIG. S9. The $^7$Li neutron momentum distribution is reconstructed using the contact values extracted in coordinate space, and compared to the VMC data

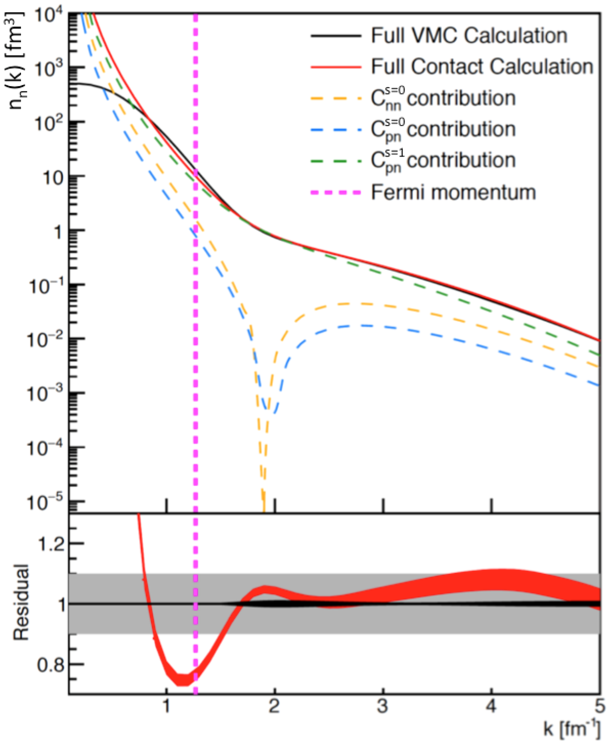


FIG. S10. The $^7$Li neutron momentum distribution is reconstructed using the contact values extracted in momentum space, and compared to the VMC data

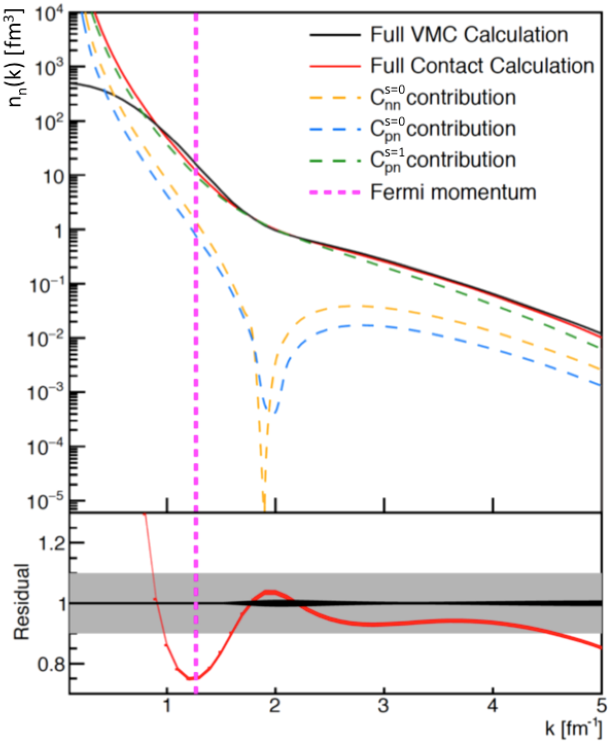


FIG. S11. The $^8$Be neutron momentum distribution is reconstructed using the contact values extracted in coordinate space, and compared to the VMC data

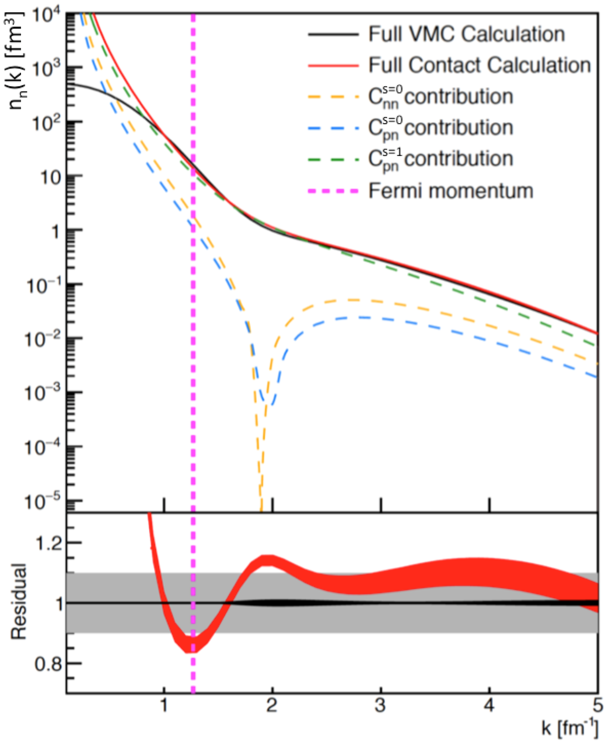


FIG. S12. The $^8$Be neutron momentum distribution is reconstructed using the contact values extracted in momentum space, and compared to the VMC data

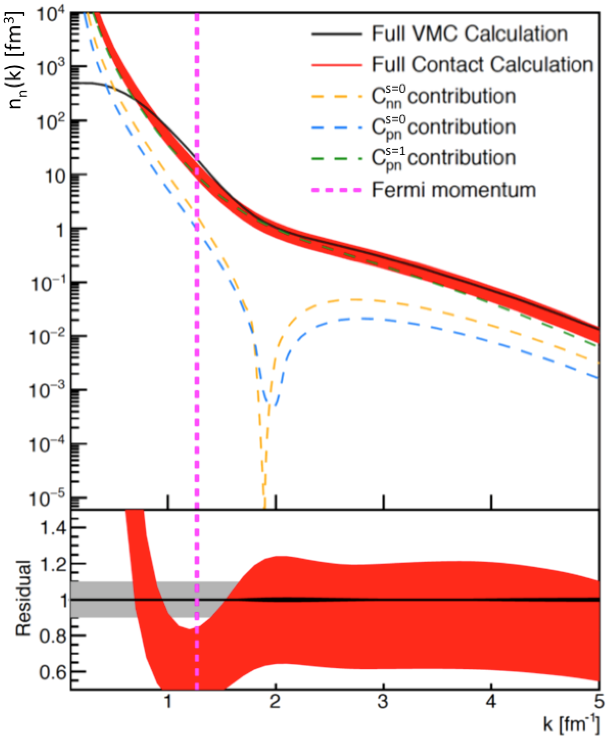


FIG. S13. The $^9$Be neutron momentum distribution is reconstructed using the contact values extracted in coordinate space, and compared to the VMC data

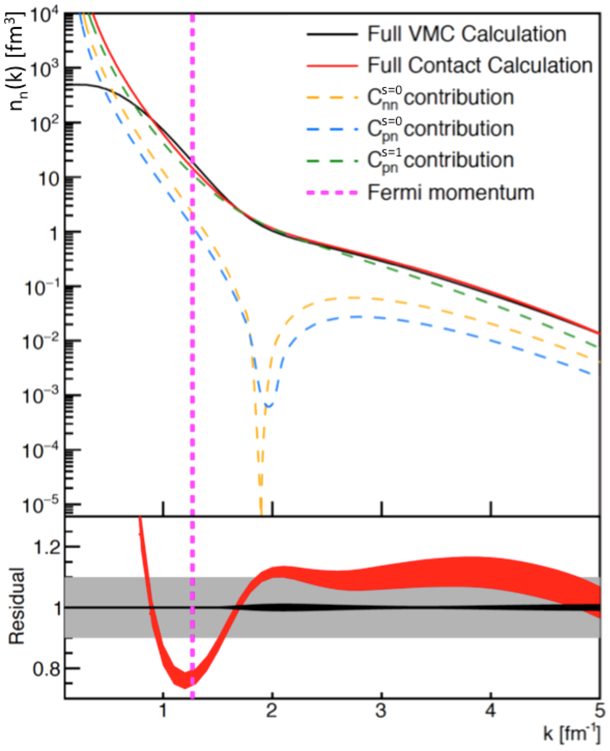


FIG. S14. The $^9$Be neutron momentum distribution is reconstructed using the contact values extracted in momentum space, and compared to the VMC data

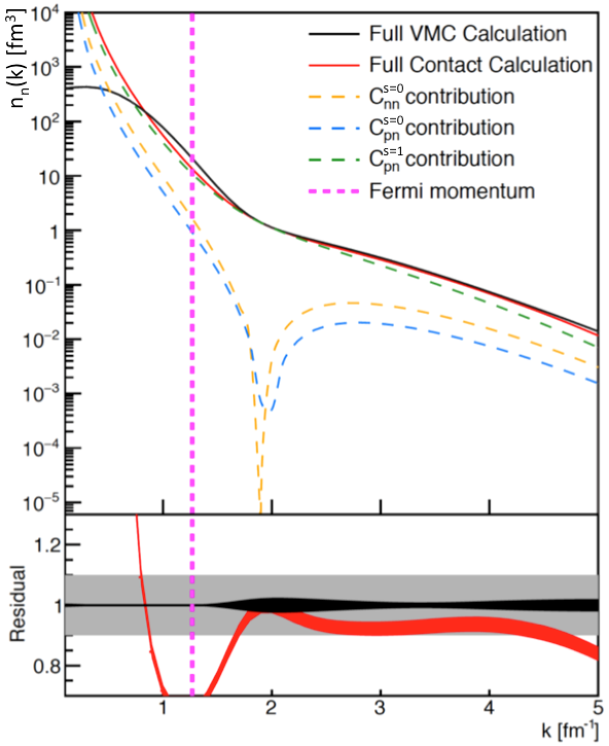


FIG. S15. The $^{10}$B neutron momentum distribution is reconstructed using the contact values extracted in coordinate space, and compared to the VMC data

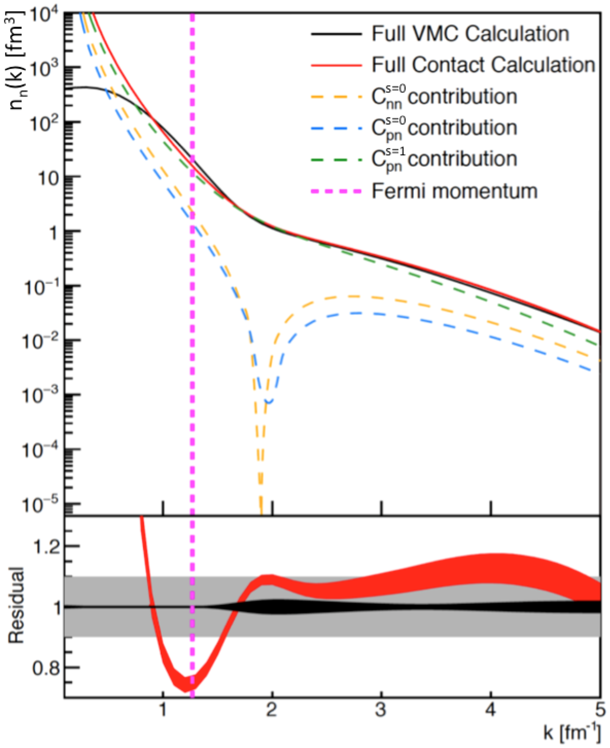


FIG. S16. The $^{10}$B neutron momentum distribution is reconstructed using the contact values extracted in momentum space, and compared to the VMC data

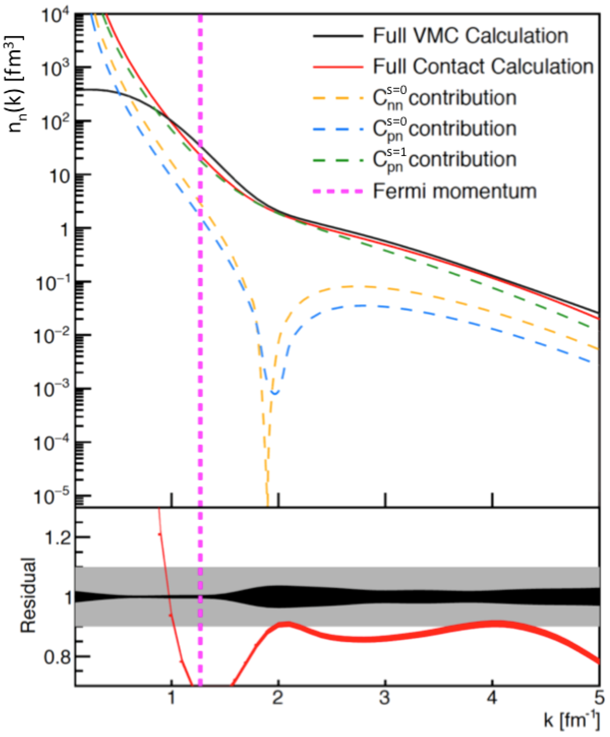


FIG. S17. The $^{12}$C neutron momentum distribution is reconstructed using the contact values extracted in coordinate space, and compared to the VMC data

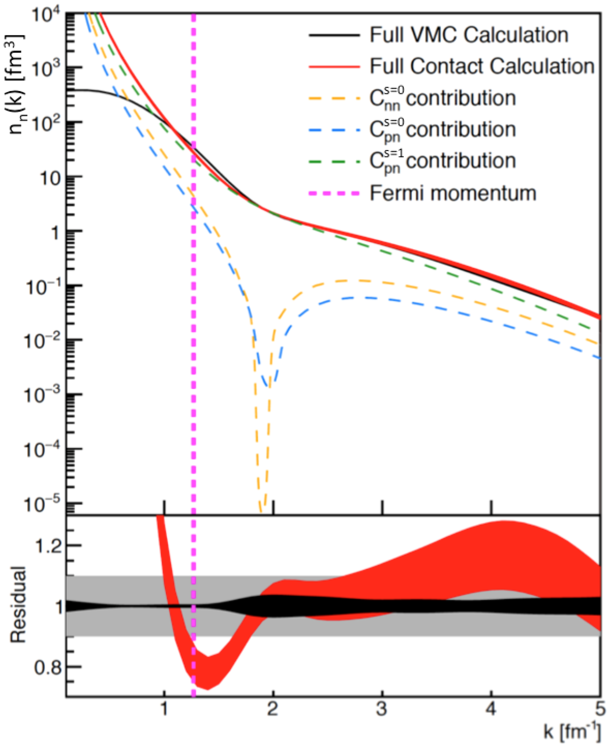


FIG. S18. The $^{12}$C neutron momentum distribution is reconstructed using the contact values extracted in momentum space, and compared to the VMC data

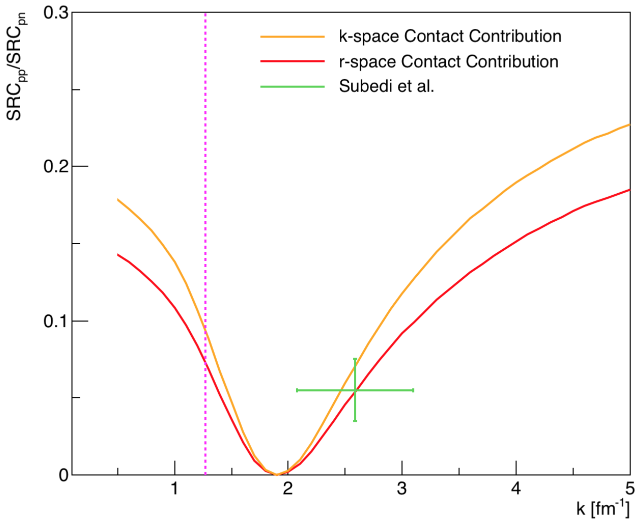


FIG. S19. The ratio between the number of $pp$ SRC pairs and $np$ SRC pairs in $^{12}C$ as a function of the relative momentum $k$, as calculated using the contact values extracted in momentum and coordinate space. The experimental data of Ref. [S3] is also presented.

[S1] R. Weiss, B. Bazak, and N. Barnea, Phys. Rev. C **92**, 054311 (2015)
[S2] R. B. Wiringa, R. Schiavilla, S. C. Pieper, and J. Carlson, Phys. Rev. C **89**, 024305 (2014).
[S3] R. Subedi *et al.*, Science **320**, 1476 (2008).
